# Supplementary material for: Sketchpose: Learning to Segment Cells with Partial Annotations
Source: arXiv:2508.17798 source file (2025-08-25)
Supplement: Supplementary file 1 [file supplementary.tex]

%!TEX root = ./sketchpose_reduced.tex

\section{Proof of the valid distance set theorem}\label{appendixA}
We start with a basic observation.
\begin{proposition}[Properties of the distance function\label{prop:distance}]\ 
\begin{itemize}
    \item $\Ac_1\subset \Ac_2 \Rightarrow \forall \xb\in \Xc, \dist(\xb,\Ac_2) \leq \dist(\xb, \Ac_1)$.
    \item $\Ac_1\subset \Ac_2$ and $\xb\in \Ac_1$ $\Rightarrow$ $\dist(\xb,\partial \Ac_1)\leq \dist(\xb,\partial \Ac_2)$.
\end{itemize}
\end{proposition}
\begin{proof}
The first item is direct:
    \begin{equation*}
         \dist(\xb,\Ac_1) = \inf_{\xb'\in \Ac_1}  \dist(\xb',\xb) \geq \inf_{\xb'\in \Ac_2} \dist(\xb',\xb) = \dist(\xb,\Ac_2).
    \end{equation*}

Here is one proof of the second iten by separating the two cases: either $x \in \mathring{\Ac_1}$ or $x \in \partial \Ac_1$. 
\begin{itemize}[leftmargin=*]
\item \emph{Case 1: $x \in \partial \Ac_1$.} This case is trivial since $\dist(\xb,\partial \Ac_1) = 0 \leq \dist(\xb,\partial \Ac_2)$ by positivity of the distance.

\item \emph{Case 2: $x \in \mathring{\Ac_1}$.} In that case, the key argument is to show that the open ball of radius $\dist(\xb,\partial \Ac_1)$ centered in $x$ is included in $\mathring{\Ac_1}$. Precisely
\begin{equation}
\label{eq:ball_in_interior}
\tilde{\Bc} \eqdef \Bc\left(x, \dist(\xb,\partial \Ac_1)\right) \subseteq \mathring{\Ac_1} \subseteq \mathring{\Ac_2}.
\end{equation}
Indeed having Equation \eqref{eq:ball_in_interior} established implies by contraposition that
\begin{equation}
\partial \Ac_2 \subseteq \mathring{\Ac_2}^c \subseteq \tilde{\Bc}^c
\end{equation}
where the first inclusion is given by $\partial \Ac_2 \eqdef \bar{\Ac_2} \setminus \mathring{\Ac_2} \subseteq \mathring{\Ac_2}^c$.
Therefore, taking infimum with respect to these sets, implies the following inequalities and by the way the intended result.
\begin{align*}
\dist(\xb,\partial \Ac_2) &= \inf_{z \in \partial \Ac_2} \| z - x\| \geq \inf_{z \in \mathring{\Ac_2}^c} \| z - x\| \\
&\geq \inf_{z \in \tilde{\Bc}^c} \| z - x\|  = \dist(\xb,\partial \Ac_1).
\end{align*}

So let's prove Equation \eqref{eq:ball_in_interior}: by contradiction, assume that there exists $z \in \tilde{\Bc} \cap \mathring{\Ac_1}^c$. 
Notice that $[x,z] \cap \mathring{\Ac_1}^c$ is a compact set (here $[x,z]$ denotes the closed segment between the points $x$ and $z$). 
Thus 
\begin{equation*}
z^* \eqdef \argmin_{x' \in [x,z] \cap \mathring{\Ac_1}^c} \| x - x'\|
\end{equation*} 
is well defined and the semi-open segment $[x, z^*[$ is included in $\mathring{\Ac_1}$. This implies that $z^* \in \partial \Ac_1$ since the sequence \mbox{$z_n \eqdef x + (1-\frac{1}{n}) \left( z^* - x\right) \in [x, z^*[ \subseteq \mathring{\Ac_1}$} converges to $z^*$. The contradiction comes from 
\begin{equation*}
\dist(\xb,\partial \Ac_1) \leq \| z^* - x\| \leq \| z - x \| < \dist(\xb,\partial \Ac_1).
\end{equation*}
The first inequality holds because $z^* \in \partial \Ac_1$, the second one because $z^* \in [x,z]$ and last one because $z \in \tilde{\Bc}$.

By proof by contradiction, Equation \eqref{eq:ball_in_interior} holds. 
\end{itemize}
In conclusion, in all cases the inequality is verified.
\end{proof}

Theorem \ref{thm:valid_dist_set} can be proven in two steps. 
    First, notice that the inclusion $\Bc \subseteq \Ec$ (Assumption \ref{ass:ass1}) and the first bullet in Proposition \ref{prop:distance} implies that $\dist(\xb, \Ec) \leq \dist(\xb,\Bc)$ for any $\xb\in \Xc$.

    Let's establish the converse inequality. Let $\xb$ denote an arbitrary point in $\Dc$. Aiming for a proof by contradiction, assume that $\dist(\xb, \Ec) < \dist(\xb, \Bc)$.
     We can proceed by separating two cases:
    \begin{itemize}[leftmargin=*]
        \item \emph{Case 1: $\dist(\xb, \Ec) = 0$}. This implies that $\xb \in \Ec$ since the set $\Ec$ is closed as a finite union of closed sets $\partial \Xc_{i,j}$. Moreover, as $\xb$ belongs to $\Dc$, in particular $\xb$ belongs to $\Sc$. It is sufficient to apply \eqref{eq:boundaries_drawn} and obtain $\xb \in \Ec \cap \Sc \subseteq \Bc$ which is inconsistent with $\dist(\xb, \Bc) > 0$. 
        \item \emph{Case 2: $r \eqdef \dist(\xb, \Ec) > 0$}. The point $\xb$ verifies $\dist(\xb, \Bc) \leq \dist(\xb, \Cc \Bc)$ as $\xb \in \Dc$. Let us define $r \eqdef \dist(\xb,\Ec) > 0$ and $\varepsilon \eqdef \dist(\xb,\Cc \Bc) - \dist(\xb,\Ec) \geq \dist(\xb,\Bc) - \dist(\xb,\Ec) > 0$ by assumption. Since $\xb$ belongs to $\Sc$, there exists $i_0 \in \{0,1\}$ such that $\xb \in \Sc_{i_0}$. Because $\dist(\xb,\Ec) = r$, there exists a point $\zb \in \Ec$ such that $r \leq \|\xb - \zb \|_2 = r + \varepsilon/2$.
    
    	\begin{itemize}[leftmargin=*]
    		\item \emph{Case 2.a: $\zb \in \Sc_{i_0}$.} By assumption \eqref{eq:boundaries_drawn}, the contradiction comes quickly since now
    		\begin{equation*}
    		\zb \in \Sc_{i_0} \cap \Ec \subseteq \Sc \cap \Ec \subseteq \Bc \subseteq \Cc \Bc,
    		\end{equation*} 
    		and this implies the contradictive inequality 
    		\begin{equation*}
    		r + \varepsilon = \dist(\xb, \Cc \Bc) \leq \|\xb-\zb\|_2 \leq r + \varepsilon/2.
\end{equation*}
    		\item \emph{Case 2.b: $\zb \notin \Sc_{i_0}$.}  In that case, we may define the point $\yb$ on the line $[\xb,\zb]$ which is the nearest from the point $\xb$ and also in $\partial \Sc_{i_0}$. Since $\yb \in \partial \Sc_{i_0} \subseteq \Cc\Bc$, it implies a contradiction as intended:
    		\begin{align*}
    		r+\varepsilon &= d(\xb, \Cc\Bc) \leq \|\xb, P(s)\|_2 \\
    		&= s \| \xb-\zb\|_2 \leq \| \xb-\zb\|_2 = r+ \varepsilon/2.
    		\end{align*}
    		The point $\yb$ is defined as $P(s)$ where the map $P : t \mapsto t\zb + (1-t) \xb$ assigns to each scalar $t \in [0,1]$ a point $P(t)$ of the line and set
    		\begin{equation*}
    		s \eqdef \inf_{P(t) \in \Sc_{i_0}} t.
			\end{equation*}
			Since $P(0) = \xb \in \Sc_{i_0}$ and $P(1) = \zb \notin \Sc_{i_0}$, the scalar $s$ is well defined. The remaining task is to show that $P(s) \in \partial \Sc_{i_0}$. The argument works by construction and with a topological argument. Indeed, by definition of the infimum, there exists a sequence $0 < \eta_n \rightarrow 0$ such that $P(s + \eta_n) \notin \Sc_{i_0}$, thus $P(s) \notin \mathring{\Sc_{i_0}}$. Also by definition, for all $0 \leq \eta < s$, $P(\eta) \in \Sc_{i_0}$, thus $P(s) \in \bar{\Sc_{i_0}}$.
    	\end{itemize}
    \end{itemize}
In both cases, the assumption $\dist(\xb, \Ec) < \dist(\xb, \Bc)$ leads to a contradiction. We deduce that $\dist(\xb, \Ec) \geq \dist(\xb, \Bc)$.

The second inequality in Theorem \ref{thm:valid_dist_set} is a consequence of the property \eqref{eq:eq_ass1}. Indeed, this property implies that we can separate the strokes $\Sc_i$ into connected components $\Sc_{i,j}$. These are subsets of the connected components $\Xc_{i,j'}$ for some $j'$ depending on $j$.
The inequality is then just a consequence of Proposition \ref{prop:distance}. 

\section{Data augmentation}\label{appendixC}

Data augmentation is one of the most expensive parts of the code. In fact, it recalculates the flows and distance maps on the fly at each iteration. In addition, for learning to converge faster, it is important to ensure that a patch always contains labels, even with partial annotations. In the original implementation, this was done recursively, i.e. by randomly selecting patches until they contained data. This method is inefficient for sparsely annotated images. Instead, we choose to randomly select centroids of patches among annotated pixels, so that the randomly selected patches are never empty. This avoids unnecessary recursive computation of the data augmentation function.

Furthermore, since data augmentation and flow calculation are not commutative, it was not possible to calculate the flows once and then apply the data augmentation. Nevertheless, it would be possible to calculate a deterministic number of data augmentations on the images in the dataset in advance, calculate the flows and then simply pick up the data using a data loader. We will explore this feature in forthcoming versions.
